# Supplementary material for: DiffusionRollout: Uncertainty-Aware Rollout Planning in Long-Horizon PDE Solving
Source: arXiv:2602.13616 source file (2026-02-14)
Supplement: Supplementary file 1 [file appendix_image_list.tex]

\midrule
\multicolumn{8}{c}{Gray-Scott~\citep{Ohana:2024TheWell}} \\
\midrule
\multicolumn{8}{c}{\includegraphics[width=\textwidth]{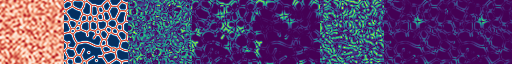}} \\
\multicolumn{8}{c}{\includegraphics[width=\textwidth]{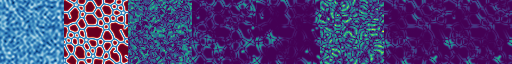}} \\
\multicolumn{8}{c}{\includegraphics[width=\textwidth]{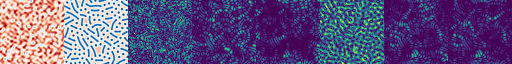}} \\
\midrule
\multicolumn{8}{c}{Turbulent Flow~\citep{Ohana:2024TheWell}} \\
\midrule
\multicolumn{8}{c}{\includegraphics[width=\textwidth]{Images/main/turbulent_i001-t095-c000.png}} \\
\multicolumn{8}{c}{\includegraphics[width=\textwidth]{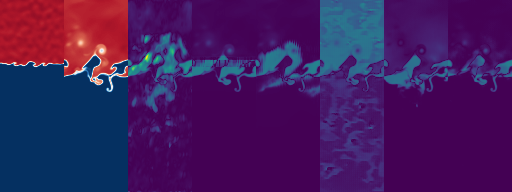}} \\
\multicolumn{8}{c}{\includegraphics[width=\textwidth]{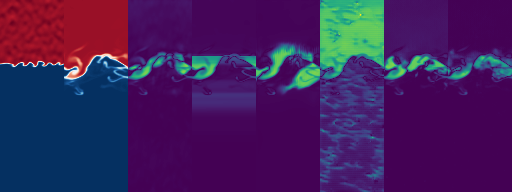}} \\
\midrule
\multicolumn{8}{c}{Cahn-Hilliard~\citep{Soares:2023Exponential}} \\
\midrule
\multicolumn{8}{c}{\includegraphics[width=\textwidth]{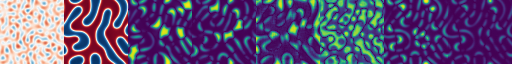}} \\
\multicolumn{8}{c}{\includegraphics[width=\textwidth]{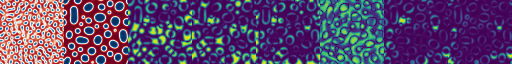}} \\
\multicolumn{8}{c}{\includegraphics[width=\textwidth]{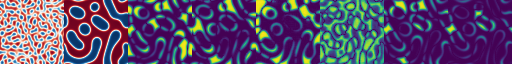}} \\
\midrule
\multicolumn{8}{c}{Anisotropic Diffusion~\citep{Koehler:2024APEBench}} \\
\midrule
\multicolumn{8}{c}{\includegraphics[width=\textwidth]{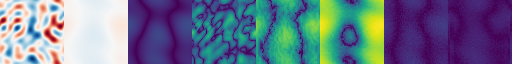}} \\
\multicolumn{8}{c}{\includegraphics[width=\textwidth]{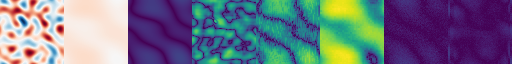}} \\
\multicolumn{8}{c}{\includegraphics[width=\textwidth]{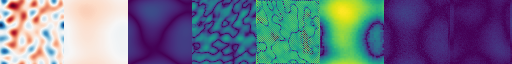}} \\
